# Supplementary material for: Word forms - not just their lengths- are optimized for efficient communication
Source: arXiv:1703.01694 source file (2017-05-31)
Supplement: Supplementary file 1 [file si.tex]

\section*{Supplementary Discussion 1: Preceding Context Revisited}
%More recently, an alternative theory has gained traction arguing that the regularity emerges from constraints relating to efficient communication: speakers may vary the length of their productions to achieve \textit{Uniform Information Density}, or UID \citep{genzelCharnaik2002, aylettTurk2004, levyJaeger2007,piantadosiEtAl2011}.
%If a word is highly predictable in context for a listener, a rational speaker should provide a shorter signal to avoid redundancy; if a word is unpredictable, a longer signal will help to avoid a sudden burst of information that could lead to a communicative failure \citep{levyJaeger2007}. 
%\citet{piantadosiEtAl2011} showed that word lengths are better predicted by average in-sentence predictability than by frequency across a broad set of European languages.

\citet{piantadosiEtAl2011} found that a word's mean predictability across contexts is a better predictor of length in characters than unigram surprisal (negative log unigram probability), consistent with the theory of Uniform Information Density. 
Here we add a substantial caveat to this observation: the correlations obtained in that study can be attributed to an interaction between in-dictionary and out-of-dictionary word types, and that this relationship is significantly weakened when each group is analyzed separately (Figure \ref{4groups_replicationPlot}).
In fact, mean trigram surprisal has no more predictive power with respect to length than unigram surprisal (negative log unigram probability) within 1) lexical items that can be found in a dictionary 2) words borrowed from English into other languages 3) words not found in any dictionary, primarily names, acronyms, and toponyms.
